# Supplementary material for: Extended Report: The Implicit Calculus
Source: arXiv:1203.4499 source file (2012-03-20)
Supplement: Supplementary file 1 [file Appendix.tex]

\appendix
\section{Proofs}

For the proof, we defined condition \disjoint{} using the following
\nonoverlap{} condition:
\begin{align*}
  & \nonoverlap(\rulet_1,\rulet_2) \defeq 
  \forall \theta. \theta \rulet_1 \ne \theta \rulet_2
  \\
  & \disjoint(\rulesetvar_1,\rulesetvar_2) \defeq 
    \forall \rulet_1 \in \rulesetvar_1.\forall \rulet_2 \in
    \rulesetvar_2. 
    \nonoverlap(\rulet_1, \rulet_2)
\end{align*}

\label{sec:appendix}

%%%%%%%%%%%%%%%%%%%%%%%%%%%%%%%%%%%%%%%%%%%%%%%%%%%%%%%%%%%%%%%%%%%%%%%%%%%%%%%%
\lempredstable

\begin{proof}

  \begin{enumerate}

  \item \label{eq:nonoverlap-stable}

    $\nonoverlap(\theta \rulet_1, \theta \rulet_2) = \forall
    \theta'. \theta' \theta \rulet_1 \ne \theta' \theta \rulet_2$ We
    can always choose $\theta''$ such that $\theta'' = \theta' \theta$
    for all $\theta'$. Then, $\theta'' \rulet_1 \ne \theta'' \rulet_2$
    is implied by $\nonoverlap(\rulet_1, \rulet_2)$.

  \item To show: $\disjoint(\rulesetvar_1, \rulesetvar_2) \implies
    \forall \theta. \disjoint(\theta \rulesetvar_1, \theta \rulesetvar_2)$
    \[
    \begin{array}{l}
      \disjoint(\rulesetvar_1, \rulesetvar_2) = 
      \forall \rulet_1 \in \rulesetvar_1.
      \forall \rulet_2 \in \rulesetvar_2. 
      \nonoverlap(\rulet_1, \rulet_2) \\
      \implies \forall \rulet_1 \in \rulesetvar_1.
      \forall \rulet_2 \in \rulesetvar_2. 
      \forall \theta. 
      \nonoverlap(\theta \rulet_1, \theta \rulet_2) \\
      \implies \forall \theta. 
      (\forall \rulet_1' \in \theta \rulesetvar_1.
      \forall \rulet_2' \in \theta \rulesetvar_2. 
      \nonoverlap(\rulet_1', \rulet_2')) \\
      = \forall \theta. 
      \disjoint(\theta \rulesetvar_1, \theta \rulesetvar_2)
    \end{array}
    \]
    The first implication holds by~\ref{eq:nonoverlap-stable}.

  \item To show: $\coherent(\env, \type) 
    \implies \forall \theta. \coherent(\theta \env, \theta \type)$
    \begin{align*}
      & \coherent(\theta \env, \theta \type) \\
      \eqv~ & \forall \theta'. 
      \theta' \lookup{(\theta \env)}{\theta \type} =
      \lookup{(\theta' \theta \env)}{\theta' \theta \type} \\
      \eqv~ & \forall \theta'. 
      \theta' \theta \lookup{\env}{\type} = \theta' \theta
      \lookup{\env}{\type}
    \end{align*}
    where $\theta' \lookup{(\theta \env)}{\theta \type} = \theta'
    \theta \lookup{\env}{\type}$ and $\lookup{(\theta' \theta
      \env)}{\theta' \theta \type} = \theta' \theta
    \lookup{\env}{\type}$ by $\coherent(\env, \type)$.
  \item 
    \begin{enumerate}
    \item To show: $\distinctwith(\rulesetexp) \implies
      \distinctwith(\overline{\relation{\theta e}{\theta \rulet}})$
      \begin{align*}
        & \distinctwith(\rulesetexp) \\
        \eqv~ & 
        \forall \myrelation{e_1}{\rulet_1}, \myrelation{e_2}{\rulet_2}
        \in \rulesetexp. \forall \theta'. \theta' \rulet_1 \neq
        \theta' \rulet_2 \\
        \implies~ & \forall \myrelation{e_1}{\rulet_1}, \myrelation{e_2}{\rulet_2}
        \in \rulesetexp. \forall \theta'. 
        \theta' \theta \rulet_1 \neq \theta' \theta \rulet_2 \\
        \implies~ &
        \forall \myrelation{e_1'}{\rulet_1'}, \myrelation{e_2'}{\rulet_2'}
        \in \overline{\relation{\theta e}{\theta \rulet}}.
        \forall \theta'. \theta' \rulet_1' \neq \theta' \rulet_2  \\
        \eqv~ & 
        \distinctwith(\overline{\relation{\theta e}{\theta \rulet}})
      \end{align*}
    \item can be shown similarly as (1).
    \item can be shown similarly as (1).
    \end{enumerate}
  \end{enumerate}
\end{proof}

%%%%%%%%%%%%%%%%%%%%%%%%%%%%%%%%%%%%%%%%%%%%%%%%%%%%%%%%%%%%%%%%%%%%%%%%%%%%%%%%
%%%%%%%%%%%%%%%%%%%%%%%%%%%%%%%%%%%%%%%%%%%%%%%%%%%%%%%%%%%%%%%%%%%%%%%%%%%%%%%%

\lemresstable{aplem:res-stable}

\begin{proof}
  We prove by induction on the derivation of static resolution.
  Suppose $\rulet = \rulesch{\alpha}{\rulesetvar}{\type}$ and
  $\env(\type) = \rulesch{\beta}{\rulesetvar'}{\type'}$. By
  the definition of predicate \coherent{}, \\
  \begin{equation*}
    (\theta \env)(\theta \type) = \theta \env(\type) = \theta
    (\rulesch{\beta}{\rulesetvar'}{\type'}) = \rulesch{\beta}{\theta
      \rulesetvar'}{\theta \type'}
  \end{equation*}
  (we assume $\dom(\theta) \cap \bar{\alpha} = \nil$ and $\dom(\theta)
  \cap \bar{\beta} = \nil$ without loss of generality). Then, $\theta
  (\rulesch{\alpha}{\rulesetvar}{\type}) = \rulesch{\alpha}{\theta
    \rulesetvar}{\theta \type}$ and 
  $\unify{\theta \type'}{\theta \type}{\bar{\beta}} =
  \unify{\type'}{\type}{\bar{\beta}}$.
  
  Now we are to show that for all $\rulet_i \in \theta' \theta
  \rulesetvar' - \theta \rulesetvar$,
  \begin{equation}
    \label{eq:res-stable-goal1}
    \theta \env \vturns \rulet_i
  \end{equation}
  where $\theta' = \unify{\type'}{\type}{\bar{\beta}}$. We know from
  the premise of \StaRes{} that $\env \vturns \rulet_i'$ for all
  $\rulet_i' \in \theta' \rulesetvar' - \rulesetvar$. Then, by
  induction hypothesis, $\theta \env \vturns \theta
  \rulet_i'$. $\theta' \theta \rulesetvar' - \theta \rulesetvar
  = \theta \theta' \rulesetvar' - \theta \rulesetvar \subseteq \theta
  (\theta' \rulesetvar' - \rulesetvar)$ and
  thus,~(\ref{eq:res-stable-goal1}) is true.

  Predicates \coherent{}, \disjoint{}, and \distinctctx{} are stable
  under substitution by~lemma \ref{aplem:pred-stable}. Therefore,
  $\theta \env \vturns \theta \rulet$.
\end{proof}

%%%%%%%%%%%%%%%%%%%%%%%%%%%%%%%%%%%%%%%%%%%%%%%%%%%%%%%%%%%%%%%%%%%%%%%%%%%%%%%%
%%%%%%%%%%%%%%%%%%%%%%%%%%%%%%%%%%%%%%%%%%%%%%%%%%%%%%%%%%%%%%%%%%%%%%%%%%%%%%%%

\lemtystable{aplem:ty-stable}

\begin{proof} We prove by induction on the typing derivation.
  \\
  \case \TyQuery~ Trivially held by lemma~\ref{aplem:res-stable}
  (Predicate \unambiguous{} is trivially stable under substitution).
  \\
  \\
  \case \TyRule~ We need to show
  \begin{equation*}
    \theta \env \turns
    \relation
    {\theta(\ruleabs{(\rulesch{\alpha}{\rulesetvar}{\type})}{e})}
    {\theta(\rulesch{\alpha}{\rulesetvar}{\type})}.
  \end{equation*}
  We assume without loss of generality that $\bar{\alpha} \cap
  \dom(\theta) = \nil$. Then,
  \begin{equation*}
    \theta \env \turns
    \relation
    {\ruleabs
      {(\rulesch{\alpha}{\theta \rulesetvar}{\theta \type})}
      {(\theta e)}}
    {\rulesch{\alpha}{\theta \rulesetvar}{\theta \type}}
  \end{equation*}
  To show this amounts to showing,
  \begin{align*}
    \theta \env, \theta \rulesetvar \turns 
    \relation{\theta e}{\theta \type},
  \end{align*}
  which is held by the assumption and induction hypothesis. Predicate
  \unambiguous{} is trivially stable under substitution.
  \\
  \\
  \case \TyInst~ By assumption,
  \begin{equation*}
    \env \turns
    \relation
    {e[\bar{\type}]}
    {[\bar{\alpha} \mapsto \bar{\type}] \rulesetvar \To 
      [\bar{\alpha} \mapsto \bar{\type}] \type},
  \end{equation*}
  and by \TyInst,
  \begin{equation}
    \env \turns \relation{e}{\rulesch{\alpha}{\rulesetvar}{\type}}
    \label{eq:tyinst-pre}
  \end{equation}
  What we need to prove is
  \begin{equation*}
    \theta \env \turns \theta 
    \relation{(e[\bar{\type}])}
    {\theta ([\bar{\alpha} \mapsto \bar{\type}]\rulesetvar \To 
      [\bar{\alpha} \mapsto \bar{\type}]\type)}
  \end{equation*}
  After distributing substitution to sub-terms, we get
  \begin{equation*}
    \theta \env \turns
    \relation{\theta e[\theta \bar{\type}]}
    {[\bar{\alpha} \mapsto \theta \bar{\type}] \theta \rulesetvar \To 
      [\bar{\alpha} \mapsto \theta \bar{\type}] \theta \type}.
  \end{equation*}
  To show this is equivalent to showing,
  \begin{equation*}
    \theta \env \turns 
    \relation{\theta e}
    {\rulesch{\alpha}{\theta \rulesetvar}{\theta \type}},
  \end{equation*}
  which is the premise of \TyInst.
  Without loss of generality, we assume $\dom(\theta) \cap
  \bar{\alpha} = \nil$. Then, this can be rewritten to
  \begin{equation*}
    \theta \env \turns 
    \relation{\theta e}
    {\theta (\rulesch{\alpha}{\rulesetvar}{\type})},
  \end{equation*}
  which is implied by (\ref{eq:tyinst-pre}) and induction hypothesis.
  \\
  \\
  \case \TyRApp~ By assumption, $\env \turns
  \relation{(\ruleapp{e}{\rulesetexp})}{\type}$, which in turn assumes
  that,
  \begin{eqnarray}
    \label{eq:tyrapp-pre1}
    \env \turns \relation{e}{\ruleset \To \type} & \\
    \label{eq:tyrapp-pre2}
    \env \turns \relation{e_i}{\rulet_i} & \text{~for all~}
    \relation{e_i}{\rulet_i} \in \rulesetexp.
  \end{eqnarray}
  \noindent
  From (\ref{eq:tyrapp-pre1}), (\ref{eq:tyrapp-pre2}) and induction
  hypothesis, 
  \begin{eqnarray}
    \label{eq:tyrapp-ind1}
    \theta \env \turns 
    \relation{\theta e}{\theta \ruleset \To \theta \type} \\
    \label{eq:tyrapp-ind2}
    \theta \env \turns \relation{\theta e_i}{\theta \rulet_i}
  \end{eqnarray}
  \noindent
  Thus, from (\ref{eq:tyrapp-ind1}), (\ref{eq:tyrapp-ind2}) and
  \TyRApp, we have
  \begin{equation*}
    \theta \env \turns
    \relation{\theta (\ruleapp{e}{\rulesetexp})}{\theta \type}
  \end{equation*}
  (Predicate \distinctwith{} is stable under substitution by
  lemma~\ref{aplem:pred-stable}).
\end{proof}

%%%%%%%%%%%%%%%%%%%%%%%%%%%%%%%%%%%%%%%%%%%%%%%%%%%%%%%%%%%%%%%%%%%%%%%%%%%%%%%%
%%%%%%%%%%%%%%%%%%%%%%%%%%%%%%%%%%%%%%%%%%%%%%%%%%%%%%%%%%%%%%%%%%%%%%%%%%%%%%%%

\lemsemstable{aplem:sem-stable}

\begin{proof} By mutual induction on the derivation of semantic typing
  of value, rule set and environment.
  \\
  \case \TyRClos~Let $v = \rclos{\rulet, e, \tstate, \rulepgmvar}$ and
  $\rulet = \rulesch{\alpha}{\pi}{\type}$. By \TyRClos,
  \begin{align}
    \label{eq:tyrclos-pre1}
    & \vtyping \relation{\rulepgmvar}{\rulesetvar'} \\
    \label{eq:tyrclos-pre2}
    & \vtyping \relation{\tstate}{\dom(\tstate)} \\
    \label{eq:tyrclos-pre3}
    & \dom(\tstate), \rulesetvar' \cup \rulesetvar \turns
    \relation{e}{\type} \\
    \label{eq:tyrclos-pre4}
    & \disjoint(\rulesetvar, \rulesetvar') \\  
    \label{eq:tyrclos-pre5}
    & \unambiguous(\rulet)
  \end{align}
  Using this, we need to show
  \begin{equation}
    \label{eq:tyrclos-goal}
    \vtyping 
    \relation{\theta \rclos{\rulet, e, \tstate, \rulepgmvar}}
    {\theta \rulet}.
  \end{equation}
  By the definition of substitution on value, \\
  $\theta \rclos{\rulet,
    e, \tstate, \rulepgmvar} = \rclos{\theta \rulet, \theta e, \theta
    \tstate, \grulepgm{\theta \rulet}{\theta v}}$. Then, proving
  (\ref{eq:tyrclos-goal}) amounts to showing the following:
  \begin{align}
    \label{eq:tyrclos-subgoal1}
    & \vtyping \relation{\theta \rulepgmvar}{\theta \rulesetvar'} \\
    \label{eq:tyrclos-subgoal2}
    & \vtyping \relation{\theta \tstate}{\dom(\theta \tstate)} \\
    \label{eq:tyrclos-subgoal3}
    & \dom(\theta \tstate), \theta \rulesetvar' \cup \theta \rulesetvar 
    \turns \relation{\theta e}{\theta \type} \\
    \label{eq:tyrclos-subgoal4}
    & \disjoint(\theta \rulesetvar, \theta \rulesetvar') \\  
    \label{eq:tyrclos-subgoal5}
    & \unambiguous(\theta \rulet)
  \end{align}
  (\ref{eq:tyrclos-subgoal1}) and (\ref{eq:tyrclos-subgoal2}) are held
  by (\ref{eq:tyrclos-pre1}) and (\ref{eq:tyrclos-pre2}),
  respectively, and induction hypothesis. (\ref{eq:tyrclos-subgoal3}) is
  held by (\ref{eq:tyrclos-pre3}) and lemma
  (\ref{aplem:ty-stable}). (\ref{eq:tyrclos-subgoal4}) is held by lemma
  (\ref{aplem:pred-stable}) and (\ref{eq:tyrclos-subgoal5}) is trivially true.
  \\
  \\
  \case \TyREnv~Trivially held by induction hypothesis.
  \\
  \\
  \case \TyRPgm~By assumption,
  \begin{align}
    \label{eq:tyrpgm-pre1}
    & \dom(\rulepgmvar) = \rulesetvar \\
    \label{eq:tyrpgm-pre2}
    & \vtyping \relation{v_i}{\rulet_i} & \text{~for all~}
    \relation{\rulet_i}{v_i} \in \rulepgmvar \\
    \label{eq:tyrpgm-pre3}
    & \distinctrs(\rulepgmvar)
  \end{align}
  By definition of function $\dom$ and (\ref{eq:tyrpgm-pre1}),
  $\dom(\theta \rulepgmvar) = \theta \dom(\rulepgmvar) = \theta
  \rulesetvar$. By (\ref{eq:tyrpgm-pre2}) and induction hypothesis,
  $\vtyping \relation{v_i'}{\rulet_i'}$ for all \\
  $\relation{\rulet_i'}{v_i'} \in \theta \rulepgmvar$. From these and
  lemma \ref{aplem:pred-stable}, we have $\vtyping \relation{\theta
    \rulepgmvar}{\theta \rulesetvar}$.
\end{proof}

%%%%%%%%%%%%%%%%%%%%%%%%%%%%%%%%%%%%%%%%%%%%%%%%%%%%%%%%%%%%%%%%%%%%%%%%%%%%%%%%
%%%%%%%%%%%%%%%%%%%%%%%%%%%%%%%%%%%%%%%%%%%%%%%%%%%%%%%%%%%%%%%%%%%%%%%%%%%%%%%%

\lemlookup{aplem:lookup}
\begin{proof}
  By the assumption and the definition of lookup on type environment,
  there should be a context $\rulesetvar$ in $\env$ such that
  $\rulesetvar(\type) = \rulet$  and
  \begin{equation}
    \label{eq:lookup-lem1}
    \rulet \in \rulesetvar \land
    (\forall \rulet' \in \rulesetvar. \rulet' \nsucc \type 
    \lor \rulet' = \rulet)
  \end{equation}
  From knowing that $\tstate$ is well-typed w.r.t. $\env$, there should be a rule
  set $\rulepgmvar$ in $\tstate$ such that $\vtyping
  \relation{\rulepgmvar}{\rulesetvar}$.
  
  Now we are to show that $\rulepgmvar(\type) = v$ for some value
  $v$. By $\TyRPgm$, $\distinctrs(\rulepgmvar)$ holds and it is restated
  as,
  \begin{equation}
    \label{eq:lookup-lem2}
    \forall \myrelation{\rulet_1}{v_1}, \myrelation{\rulet_2}{v_2} \in
    \rulepgmvar. \forall \theta. \theta \rulet_1 \neq \theta \rulet_2 
  \end{equation}
  From~(\ref{eq:lookup-lem1}) and~(\ref{eq:lookup-lem2}), we conclude
  \begin{equation*}
    \relation{\rulet}{v} \in \rulepgmvar \land
    (\forall \relation{\rulet'}{v'} \in \rulepgmvar. 
    \rulet' \nsucc \type \lor 
    \relation{\rulet'}{v'} = \relation{\rulet}{v})
  \end{equation*}  
  which is the exact condition for $\rulepgmvar(\type) = v$ to hold.
\end{proof}

%%%%%%%%%%%%%%%%%%%%%%%%%%%%%%%%%%%%%%%%%%%%%%%%%%%%%%%%%%%%%%%%%%%%%%%%%%%%%%%%
%%%%%%%%%%%%%%%%%%%%%%%%%%%%%%%%%%%%%%%%%%%%%%%%%%%%%%%%%%%%%%%%%%%%%%%%%%%%%%%%

\lemrespreserve{aplem:res-preserve}

\begin{proof} 
  We prove by induction on the derivation of static
  resolution.
  \\
  \case \StaRes~ We first show that if static resolution succeeds,
  then dynamic resolution also succeeds. Let $\rulet =
  \rulesch{\alpha}{\rulesetvar}{\type}$ and $\env(\type) =
  \rulesch{\beta}{\rulesetvar'}{\type'}$. By lemma~\ref{aplem:lookup},
  \begin{equation}
    \tstate(\type) = v' ~\land 
    \vtyping \relation{v'}{\rulesch{\beta}{\rulesetvar'}{\type'}}
    \label{eq:respreserve-lem1}
  \end{equation}
  By induction hypothesis, 
  \begin{equation}
    \forall \rulet_i \in \theta \rulesetvar' - \rulesetvar.
    \env \vturns \rulet_i \eval v_i ~\land 
    \vtyping \relation{v_i}{\rulet_i}
    \label{eq:respreserve-lem2}
  \end{equation}
  where $\theta = \unify{\type'}{\type}{\bar{\beta}}$. Then, from
  (\ref{eq:respreserve-lem1}) and (\ref{eq:respreserve-lem2}), dynamic
  resolution succeeds.

  Next, we prove $\vtyping \relation{v}{\rulet}$ by showing each
  premise of \TyRClos{} satisfied one by one. Let $v' =
  \rclos{\rulesch{\beta}{\rulesetvar'}{\type'}, e', \tstate',
    \rulepgmvar'}$. Since
  $\vtyping \relation{v'}{\rulesch{\beta}{\rulesetvar'}{\type'}}$, we have
  \begin{align}
    \label{eq:respreserve-lem3}
    & \vtyping \relation{\rulepgmvar'}{\rulesetvar''} \\
    \label{eq:respreserve-lem4}
    & \vtyping \relation{\tstate'}{\dom(\tstate')} \\
    \label{eq:respreserve-lem5}
    & \dom(\tstate'); \rulesetvar' \cup \rulesetvar'' \turns
    \relation{e'}{\type'} \\
    \label{eq:respreserve-lem6}
    & \disjoint(\rulesetvar', \rulesetvar'') \\
    \label{eq:respreserve-lem7}
    & \unambiguous(\rulesch{\beta}{\rulesetvar'}{\type'})
  \end{align}
  
  \begin{itemize}

  \item $\vtyping \relation{\rulepgm \cup \theta
      \rulepgmvar'}{\ruleset \cup \theta \rulesetvar''}$ \\
    By (\ref{eq:respreserve-lem2}) and (\ref{eq:respreserve-lem3}), we
    know
    \begin{equation*}
      \forall \relation{\rulet_j}{v_j} \in \rulepgm \cup \theta
      \rulepgmvar'. \vtyping \relation{v_j}{\rulet_j}
    \end{equation*}
    We only need to prove $\distinctrs(\rulepgm \cup \theta
    \rulepgmvar')$. Since $\ruleset$ is a subset of $\theta
    \rulesetvar'$, $\ruleset$ and $\theta \rulesetvar''$ are
    disjoint. Also $\ruleset$ is distinct by assumption. Therefore, 
    $\distinctrs(\rulepgm \cup \theta \rulepgmvar')$ is true.

  \item $\vtyping \relation{\tstate'}{\dom(\theta \tstate')}$ \\
    Trivially held by (\ref{eq:respreserve-lem4}) and
    lemma~\ref{aplem:sem-stable}. 

  \item $\dom(\theta \tstate'); 
    \rulesetvar \cup \ruleset \cup \theta \rulesetvar''
    \turns \relation{\theta e'}{\type}$ \\
    By lemma~\ref{aplem:ty-stable} and (\ref{eq:respreserve-lem5}),
    \begin{equation}
      \label{eq:respreserve-lem8}
      \dom(\theta \tstate'); 
      \theta \rulesetvar' \cup \theta \rulesetvar'' 
      \turns \relation{\theta e'}{\theta \type'}
    \end{equation}
    We know that $\theta \rulesetvar' = \rulesetvar \cup \ruleset$ and
    $\theta \type' = \type$. Thus, we can rewrite
    (\ref{eq:respreserve-lem8}) to
    \begin{equation*}
      \dom(\theta \tstate'); 
      \rulesetvar \cup \ruleset \cup \theta \rulesetvar''
      \turns \relation{\theta e'}{\type}
    \end{equation*}

  \item $\disjoint(\rulesetvar, \ruleset \cup \theta \rulesetvar'')$\\
    Trivially held by (\ref{eq:respreserve-lem6}) and
    $\disjoint(\rulesetvar, \ruleset)$.

  \item $\unambiguous(\rulet)$ \\
    Trivially held by assumption.

  \end{itemize}
\end{proof}

%%%%%%%%%%%%%%%%%%%%%%%%%%%%%%%%%%%%%%%%%%%%%%%%%%%%%%%%%%%%%%%%%%%%%%%%%%%%%%%%
%%%%%%%%%%%%%%%%%%%%%%%%%%%%%%%%%%%%%%%%%%%%%%%%%%%%%%%%%%%%%%%%%%%%%%%%%%%%%%%%

\lemtypreserve{aplem:ty-preserve}

\begin{proof} By induction on the evaluation derivation and
  case analysis on the final rule of the typing derivation. The final
  rule of the evaluation derivation uniquely determines the final rule
  of the typing derivation since both semantics rules and typing rules
  are syntax-directed.
  \\
  \\
  \case \OpQuery~Trivially held by lemma~\ref{aplem:res-preserve}.
  \\
  \\
  \case \OpRule~By assumption,
  \begin{align}
    \tstate \turns \ruleabs{\rulet}{e} & \eval \rclos{\rulet, e,
      \tstate, \nil} \nonumber \\
    \label{eq:tyrule}
    \env \turns \relation{\ruleabs{\rulet}{e}&}{\rulet}
  \end{align}
  By \TyRule~and (\ref{eq:tyrule}), we have 
  \begin{equation}
    \label{eq:tyrule-pre1}
    \env, \rulesetvar \turns \relation{e}{\type}
  \end{equation}
  where $\rulet = \rulesch{\alpha}{\rulesetvar}{\type}$. Then, by
  (\ref{eq:tyrule-pre1}) and the assumption of well-typed environment,
  we have
  \begin{equation*}
    \vtyping \relation{\rclos{\rulet, e, \tstate, \nil}}{\rulet}
  \end{equation*}
  ($\disjoint(\rulesetvar, \nil)$ is trivially held and
  $\unambiguous(\rulet)$ is true by assumption)
  \\
  \\
  \case \OpInst~By assumption,
  \begin{align}
    \label{eq:opinst}
    & \tstate \turns e[\bar{\type}] \eval 
    [\bar{\alpha} \mapsto \bar{\type}]
    \rclos{\rulesetvar \To \type, e', \tstate', \rulepgmvar'} \\
    \label{eq:tyinst}
    & \env \turns \relation{e[\bar{\type}]}
    {[\bar{\alpha} \mapsto \bar{\type}] (\rulesetvar \To \type)}
  \end{align}
  By (\ref{eq:opinst}) and \OpInst,
  \begin{equation}
    \label{eq:opinst-pre}
    \tstate \turns e \eval 
    \rclos{\rulesch{\alpha}{\rulesetvar}{\type},
      e', \tstate', \rulepgmvar'}
  \end{equation}
  By (\ref{eq:tyinst}) and \TyInst,
  \begin{equation}
    \label{eq:tyinst-pre2}
    \env \turns \relation{e}{\rulesch{\alpha}{\rulesetvar}{\type}}
  \end{equation}
  Then, by (\ref{eq:opinst-pre}), (\ref{eq:tyinst-pre2}) and induction
  hypothesis,
  \begin{equation*}
    \vtyping \relation
    {\rclos{\rulesch{\alpha}{\rulesetvar}{\type}, 
        e', \tstate', \rulepgmvar'}}
    {\rulesch{\alpha}{\rulesetvar}{\type}},
  \end{equation*}
  which leads to the following:
  \begin{align}
    \label{eq:inst-tyrclos-pre1}
    & \vtyping \relation{\rulepgmvar'}{\rulesetvar'} \\
    \label{eq:inst-tyrclos-pre2}
    & \vtyping \relation{\tstate'}{\dom(\tstate')} \\
    \label{eq:inst-tyrclos-pre3}
    & \dom(\tstate'); \rulesetvar \cup \rulesetvar' 
    \turns \relation{e'}{\type} \\
    \label{eq:inst-tyrclos-pre4}
    & \disjoint(\rulesetvar, \rulesetvar') \\
    \label{eq:inst-tyrclos-pre5}
    & \unambiguous(\rulesch{\alpha}{\rulesetvar}{\type})
  \end{align}

  Let $\theta = [\bar{\alpha} \mapsto \bar{\type}]$. We need to prove
  \begin{equation*}
    \vtyping 
    \relation
    {\theta \rclos{\rulesetvar \To \type,
        e', \tstate', \rulepgmvar'}}
    {\theta (\rulesetvar \To \type)}
  \end{equation*}
  which amounts to showing 
  \begin{align}
    \label{eq:inst-tyrclos-goal1}
    & \vtyping \relation{\theta \rulepgmvar'}{\theta \rulesetvar'} \\
    \label{eq:inst-tyrclos-goal2}
    & \vtyping \relation{\theta \tstate'}{\dom(\theta \tstate')} \\
    \label{eq:inst-tyrclos-goal3}
    & \dom(\theta \tstate'); \theta \rulesetvar \cup 
    \theta \rulesetvar' \turns \relation{\theta e'}{\theta \type} \\
    \label{eq:inst-tyrclos-goal4}
    & \disjoint(\theta \rulesetvar, \theta \rulesetvar') \\
    \label{eq:inst-tyrclos-goal5}
    & \unambiguous(\theta \rulesetvar \To \theta \type)
  \end{align}
  (\ref{eq:inst-tyrclos-goal1}) and (\ref{eq:inst-tyrclos-goal2}) are
  true by (\ref{eq:inst-tyrclos-pre1}), (\ref{eq:inst-tyrclos-pre2})
  and lemma~\ref{aplem:sem-stable}. (\ref{eq:inst-tyrclos-goal3}) is
  held by (\ref{eq:inst-tyrclos-pre3}) and
  lemma~\ref{aplem:ty-stable}. (\ref{eq:inst-tyrclos-goal4}) is held by
  (\ref{eq:inst-tyrclos-pre4}) and
  lemma~\ref{aplem:pred-stable}. (\ref{eq:inst-tyrclos-goal5}) is
  trivially true by (\ref{eq:inst-tyrclos-pre5}).
  \\
  \\
  \case \OpRApp~By assumption,
  \begin{align*}
    & \tstate \turns \ruleapp{e}{\rulesetexp} \eval v \\ 
    & \env \turns \relation{\ruleapp{e}{\rulesetexp}}{\type}
  \end{align*}
  By inversion of these,
  \begin{align}
    \label{eq:rapp-oprapp-pre1}
    & \tstate \turns e \eval 
    \rclos{\ruleset \To \type, e', \tstate', \rulepgmvar'} \\
    \label{eq:rapp-tyrapp-pre1}
    & \env \turns \relation{e}{\ruleset \To \type} \\ \nonumber \\
    \label{eq:rapp-oprapp-pre2}
    & \tstate \turns e_i \eval v_i  \text{~for all~}
    \relation{e_i}{\rulet_i} \in \rulesetexp \\
    \label{eq:rapp-tyrapp-pre2}
    & \env \turns \relation{e_i}{\rulet_i} \text{~for all~}
    \relation{e_i}{\rulet_i} \in \rulesetexp \\ \nonumber \\
    \label{eq:rapp-oprapp-pre3}
    & \tstate', \rulepgm \cup \rulepgmvar' \turns e' \eval v \\
    \label{eq:rapp-tyrapp-pre3}
    & \distinctwith(\rulesetexp)
  \end{align}
  By (\ref{eq:rapp-oprapp-pre1}), (\ref{eq:rapp-tyrapp-pre1}) and induction
  hypothesis,
  \begin{equation*}
    \vtyping \relation
    {\rclos{\ruleset \To \type, e', \tstate', \rulepgmvar'}}
    {\ruleset \To \type},
  \end{equation*}
  by which we also have
  \begin{align}
    \label{eq:rapp-tyrclos-pre1}
    & \vtyping \relation{\rulepgmvar'}{\rulesetvar'} \\
    \label{eq:rapp-tyrclos-pre2}
    & \dom(\tstate'); \ruleset \cup \rulesetvar' 
    \turns \relation{e'}{\type} \\
    \label{eq:rapp-tyrclos-pre3}
    & \vtyping \relation{\tstate'}{\dom(\tstate')} \\
    \label{eq:rapp-tyrclos-pre4}
    & \disjoint(\ruleset, \rulesetvar')
  \end{align}
  Then, we can prove $\vtyping \relation{v}{\type}$ by
  (\ref{eq:rapp-oprapp-pre3}), (\ref{eq:rapp-tyrclos-pre2}) and induction
  hypothesis if we show
  \begin{equation}
    \label{eq:oprapp-goal}
    \vtyping \relation{(\tstate'; \rulepgm \cup \rulepgmvar')}
    {(\dom(\tstate'); \ruleset \cup \rulesetvar')}
  \end{equation}
  By (\ref{eq:rapp-oprapp-pre2}), (\ref{eq:rapp-tyrapp-pre2}) and
  induction hypothesis, we prove $\vtyping
  \relation{\rulepgm}{\ruleset}$ ((\ref{eq:rapp-tyrapp-pre3}) implies
  $\distinctrs(\rulepgm)$). Since $\ruleset$ and $\rulesetvar'$ are
  disjoint (by (\ref{eq:rapp-tyrclos-pre4})), there is no $\rulet_1$
  in $\ruleset$ such that for some $\rulet_2$ in $\rulesetvar'$ and
  $\theta$, $\theta \rulet_1$ = $\theta \rulet_2$. Thus,
  $\distinctrs(\rulepgm \cup \rulepgmvar')$
  \begin{equation}
    \vtyping \relation{(\rulepgm \cup \rulepgmvar')}
    {(\ruleset \cup \rulesetvar')}\label{eq:rapp-lem1}
  \end{equation}
  Therefore, (\ref{eq:oprapp-goal}) is true by
  (\ref{eq:rapp-tyrclos-pre3}) and (\ref{eq:rapp-lem1}).
  
\end{proof}

%%%%%%%%%%%%%%%%%%%%%%%%%%%%%%%%%%%%%%%%%%%%%%%%%%%%%%%%%%%%%%%%%%%%%%%%%%%%%%%%
%%%%%%%%%%%%%%%%%%%%%%%%%%%%%%%%%%%%%%%%%%%%%%%%%%%%%%%%%%%%%%%%%%%%%%%%%%%%%%%%

\thmsoundness

\begin{proof}
  Trivially held by lemma \ref{aplem:ty-preserve}, since $\vtyping
  \relation{\nil}{\nil}$.
\end{proof}

%%%%%%%%%%%%%%%%%%%%%%%%%%%%%%%%%%%%%%%%%%%%%%%%%%%%%%%%%%%%%%%%%%%%%%%%%%%%%%%%
%%%%%%%%%%%%%%%%%%%%%%%%%%%%%%%%%%%%%%%%%%%%%%%%%%%%%%%%%%%%%%%%%%%%%%%%%%%%%%%%

\lemtrestypreserve{aplem:trres-preserve}
\begin{proof}
  We prove by induction on the derivation of \TrRes. Let $\rulet =
  \rulesch{\alpha}{\rulesetvar}{\type}$ and 
  $\denv(\type) =
  \relation{\rulesch{\beta}{\rulesetvar'}{\type'}}{y}$. By the
  definition of function $|\cdot|$,
  \begin{equation*}
    |\denv| \turns \relation{y}{\forall \beta. |\rulesetvar'| \to |\type'|}
  \end{equation*}
  By \TyTyApp,
  \begin{align*}
    & |\denv| \turns \relation{y~\theta \bar{\beta}}
    {\subst{\bar{\beta}}{\theta \bar{\beta}} (|\rulesetvar'| \to
      |\type'|)} \\
    \eqv~ & |\denv| \turns \relation{y~\theta \bar{\beta}}
    {(|\theta \rulesetvar'| \to |\type|)}
  \end{align*}
  where $\theta = \unify{\type'}{\type}{\bar{\beta}}$ and $\type =
  \theta \type'$. \\
  By induction hypothesis and the definition of function $|\cdot|$,
  \begin{equation*}
    |\denv| \turns \relation{E_i}{\rulet_i}
  \end{equation*}
  for all $\rulet_i$ in $\theta \rulesetvar'$. Thus, by \TyApp,
  \begin{equation*}
    |\denv| \turns \relation{y~\theta \bar{\beta}~\bar{E}}
    {|\type|}
  \end{equation*}
  Therefore, $|\denv| \turns \Lambda \bar{\alpha}.\lambda(\bar{x} :
  |\rulesetvar|).(y~\theta \beta~\bar{E})$, by applying \TyAbs{} and
  \TyTyAbs{}.

\end{proof}

\lemtranstypreserve{aplem:tr-preserve}
\begin{proof}
  We prove by induction on the derivation of translation.
  \\
  \case \TrQuery~Trivially held by lemma~\ref{aplem:trres-preserve}.
  \\
  \\
  \case \TrRule~Let $\type = \rulesch{\alpha}{\ruleset}{\type}$. By
  assumption,
  \begin{equation*}
    \denv \turns 
    \relation{\ruleabs{\rulet}{e}}{\rulet} \leadsto
    \Abs{\bar{\alpha}}{\abs{({\relation{\bar{x}}{|\bar{\rulet}|}})}{E}}
  \end{equation*}
  which leads to,
  \begin{equation*}
    \denv; \overline{\relation{\rulet}{x}} \turns 
    \relation{e}{\type} \leadsto E
  \end{equation*}
  From this and induction hypothesis,
  \begin{equation*}
    |\denv| \cup \overline{\relation{x}{|\rulet|}} \turns 
    \relation{E}{|\type|}
  \end{equation*}
  Therefore, by \TyAbs{} and \TyTyAbs,
  \begin{equation*}
    |\denv| \turns \relation
    {\Abs{\bar{\alpha}}{\abs{({\relation{\bar{x}}{|\bar{\rulet}|}})}{E}}}
    {\forall \bar{\alpha}.|\ruleset| \to |\type|}
  \end{equation*}
  \\
  \case \TrInst~By assumption,
  \begin{equation*}
    \denv \turns \relation{e[\bar{\type}]}{\theta (\rulesetvar \to
      \type)} \leadsto E~|\bar{\type}|
  \end{equation*}
  where $\theta = \subst{\bar{\alpha}}{\bar{\type}}$. By $\TrInst$,
  \begin{equation*}
    \denv \turns \relation{e}{\rulesch{\alpha}{\ruleset}{\type}}
      \leadsto E
  \end{equation*}
  From this and induction hypothesis,
  \begin{equation*}
    |\denv| \turns \relation{E}{\forall \bar{\alpha}. |\ruleset| \to |\type|}
  \end{equation*}
  Therefore, by \TyTyApp,
  \begin{equation*}
    |\denv| \turns \relation{E~|\bar{\type}|}
    {|\theta \ruleset| \to |\theta \type|}
  \end{equation*}
  \\
  \case \TrRApp~By assumption,
  \begin{align*}
    & \denv \turns \relation{e}{\ruleset \To \type} \leadsto E \\
    & \denv \turns \relation{e_i}{\rulet_i} \leadsto E_i~\text{for
      all}~ \relation{e_i}{\rulet_i} \in \rulesetexp
  \end{align*}
  From these and induction hypothesis,
  \begin{align*}
    & |\denv| \turns \relation{E}{|\ruleset| \to |\type|} \\
    & |\denv| \turns \relation{E_i}{|\rulet_i|}
  \end{align*}
  where $|\ruleset| = |\rulet_1| \to \cdots \to
  |\rulet_n|$. \\
  Therefore, by \TyApp,
  \begin{equation*}
    |\denv| \turns \relation{E~\bar{E}}{|\type|}
  \end{equation*}
\end{proof}

\thmtranstypreserve
\begin{proof}
  Trivially held by lemma~\ref{aplem:tr-preserve}.
\end{proof}

\section{Unification}
\label{sec:unification}

\figtwocol{fig:unify}{Unification}{
\small

\bda{lc}
\multicolumn{2}{l}{
  \myruleform{\unify{\tau_1}{\tau_2}{\bar{\alpha}} = \theta}}
\\ \\

& \myirule{\alpha \not\in \bar{\alpha}}{\unify{\alpha}{\alpha}{\bar{\alpha}} = \varnothing}  \\

& \myirule{\alpha \in \bar{\alpha}}{\unify{\tau}{\alpha}{\bar{\alpha}} = [\alpha \mapsto \tau]} 
\quad\quad 
\myirule{\alpha \in \bar{\alpha}}{\unify{\tau}{\alpha}{\bar{\alpha}} = [\alpha \mapsto \tau]} \\ \\

& \myirule
{
  \mid\!\overline{\alpha_1}\!\mid = \mid\!\overline{\alpha_2}\!\mid \quad\quad
  \theta_1 \overset{\tt let}{=} [\overline{\alpha_1} \mapsto \overline{\alpha_2}] \\
  \unify{\theta_1 \tau_1}{\tau_2}{\bar{\alpha}} = \theta_2 \quad\quad
  \unify{\theta_2 \theta_1 \rulesetvar_1}{\theta_2 \rulesetvar_2}{\bar{\alpha}} = \theta_3

}
{
  \unify
    {\forall \overline{\alpha_1}. \rulesetvar_1 \Rightarrow \tau_1}
    {\forall \overline{\alpha_2}. \rulesetvar_2 \Rightarrow \tau_2}{\bar{\alpha}} 
  = \theta_3 \theta_2 \theta_1
} \\ \\

\multicolumn{2}{l}{
  \myruleform{
    \unify{\rulesetvar_1}{\rulesetvar_2}{\bar{\alpha}} = \theta}}
\\ \\

& \myirule
{ \{a,b\} = \{1,2\} \quad\quad
  \rulesetvar_{a,1} = \{ \rulet \} \\ \rulesetvar_{b,1} = \{ \rulet_1,\ldots,\rulet_n \} \quad (n \geq 1)
  \quad\quad \theta_0 = \varnothing \\
  \unify{\theta_{i-1} \cdots \theta_1\rulet}
        {\theta_{i-1} \cdots \theta_1\rulet_i}
        {\bar{\alpha}} = \theta_{i} \quad (\forall i \in [1,n]) \\
  \unify{\theta_{n} \cdots \theta_1\rulesetvar_{1,2}}
        {\theta_{n} \cdots \theta_1\rulesetvar_{2,2}}
        {\bar{\alpha}} = \theta
}
{
  \unify
    {\rulesetvar_{1,1} \uplus \rulesetvar_{1,2}}
    {\rulesetvar_{2,1} \uplus \rulesetvar_{2,2}}
    {\bar{\alpha}} 
  = \theta\theta_{n} \cdots \theta_1
} 
\\ \\
& {
  \unify
    {\varnothing}
    {\varnothing}{\bar{\alpha}} 
  = \varnothing
} 
\eda
}

\section{Substitution}
\label{sec:substitution}

\figtwocol{fig:subst}{Substitutions} {
\scriptsize

\bda{l}
\substone \beta = 
\left\{
  \begin{array}{lr}
    \type & \beta = \alpha \\
    \beta & \text{otherwise}
  \end{array}
\right.
\\
\substone \rulet =
\left\{
    \
    \begin{array}{lr}
      \rulet' & \alpha \notin \bar{\alpha} \\
      \rulet & \text{otherwise}
    \end{array}
\right. \\
\quad\quad\text{~where~}
\rulet = \rulesch{\alpha}{\rulesetvar}{\type'} \\
\quad\quad\quad\quad\quad
\rulet' = 
\rulesch{\alpha}
{(\substone \rulesetvar)}
{(\substone \type')} \\ \\

\substone \rulesetvar =
\myset{ \substone \rulet ~\mid~ \rulet \in \rulesetvar }
\\ \\

\substone ?\rulet = ?(\substone \rulet) \\ 

\substone \ruleabs{\rulet}{e} =
\left\{
    \
    \begin{array}{lr}
      \ruleabs
      {(\substone \rulet)}{([ \alpha \mapsto \type] e)} &
      \alpha \notin \bar{\alpha} \\
      \ruleabs{\rulet}{e} & \text{otherwise}
    \end{array}
\right.\\
\quad\quad\text{~where~}
\rulet = \rulesch{\alpha}{\rulesetvar}{\type'} \\

\substone e[\bar{\type}] =
(\substone e)[\substone \bar{\type}] \\

\substone 
\ruleapp{e}{\rulesetexp} = \\
\quad\quad
\ruleapp{(\substone e)}
{\overline{\relation
    {\substone e}
    {\substone \rulet}}}
\\ \\

\substone \rclos{\rulet, e, \tstate, \rulepgmvar} = \\
\left\{
\begin{array}{lr}
\rclos{
  \substone \rulet, 
  \substone e, 
  \substone \tstate, 
  \substone \rulepgmvar}
& \alpha \notin \bar{\alpha} \\

\rclos{\rulet, e, \substone \tstate, \rulepgmvar}
& \text{~otherwise}
\end{array}
\right. \\
\quad\quad\text{~where~}
\rulet = \rulesch{\alpha}{\rulesetvar}{\type'} 
\\ \\

\substone \rulepgmvar =
\myset{
  (\relation
  {\substone \rulet}
  {\substone v}) ~\mid~ \relation{\rulet}{v} \in \rulepgmvar }
\\ \\

\substone \cdot = \cdot \\
\substone \tstate; \rulepgmvar = 
(\substone \tstate); (\substone \rulepgmvar)

\eda

}

\section{Typing Rules of System F}
\label{sec:substitution}

\figtwocol{fig:systemf}{Typing rules of System F}{
\small
\bda{lc} 

\multicolumn{2}{l}{\myruleform{\env \turns \relation{E}{T}}} \\ \\

\TyVar &
\myirule
{ \env(x) = T}
{ \env \turns \relation{x}{T} }
\\ \\

\TyAbs &
\myirule
{ \env + \relation{x}{T_1} \turns \relation{E}{T_2} }
{ \env \turns \relation{\lambda (\relation{x}{T}). E}{T_1 \to T_2}
} 
\\ \\

\TyApp &
\myirule
{ \env \turns \relation{E_1}{T_2 \to T_1} \\
  \env \turns \relation{E_2}{T_2}
}
{ \env \turns \relation{E_1\;E_2}{T_1} }
\\ \\

\TyTyAbs &
\myirule
{ \env \turns \relation{e}{T}
}
{ \env \turns \relation{\Lambda \alpha. E}{\forall \alpha. T} }
\\ \\

\TyTyApp &
\myirule
{ \env \turns \relation{E}{\forall \alpha. T'} }
{ \env \turns \relation{E\;T}{\subst{\alpha}{T} T'} }
\\ \\

\TyUnit &
\env \turns \relation{()}{()}

\eda
}

%%% Local Variables: 
%%% mode: latex
%%% TeX-master: "../Main"
%%% End: 
